# Supplementary material for: Probing new physics in $B_s \to (K,K^*)\tau \nu$ and $B \to \pi \tau \nu$ decays
Source: arXiv:1908.06244 source file (2019-08-17)

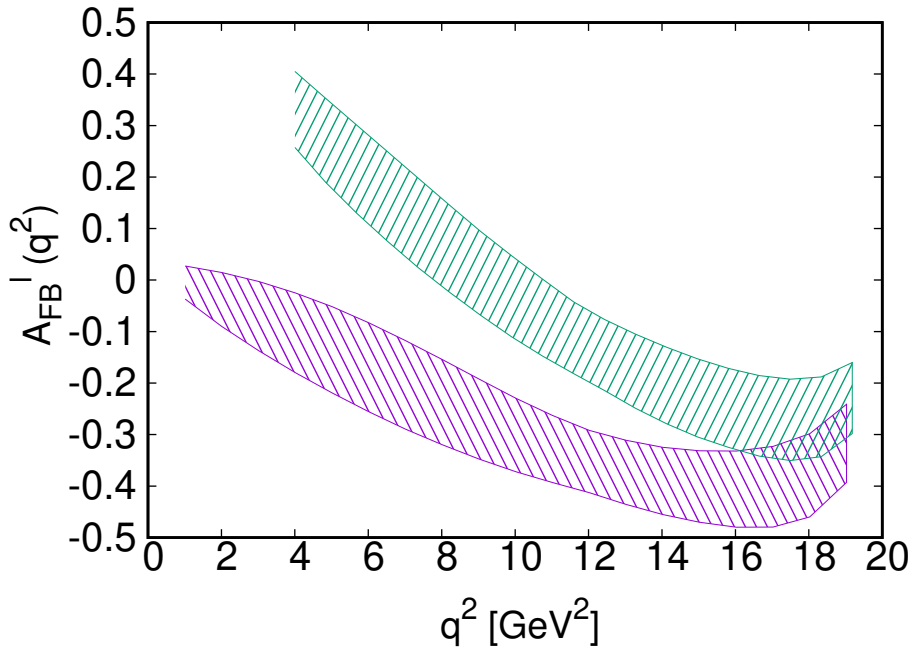

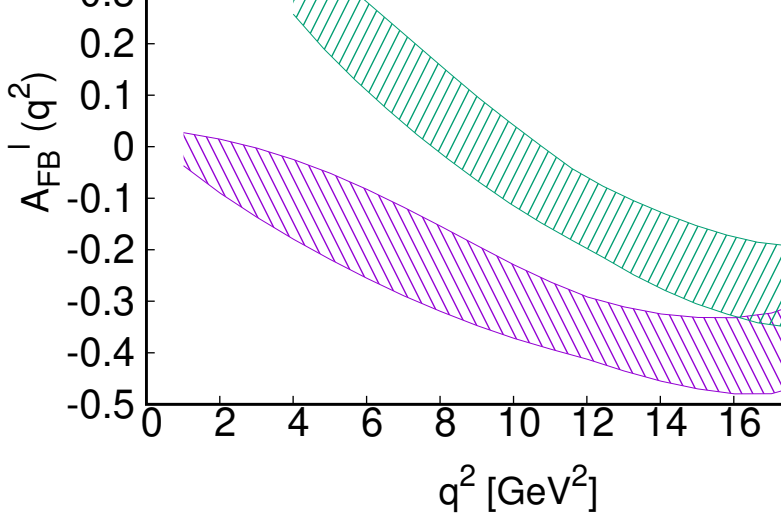

Supplement: Supplementary file 3 [file q2_afbmutaubskst_sm-eps-converted-to.pdf]
